# Supplementary material for: Dynamical Jahn-Teller effects on the generation of electronic ring currents by circularly polarized light
Source: arXiv:2105.10449 source file (2021-05-21)
Supplement: Supplementary file 1 [file ecurrents_SI.pdf]

# Supporting Information:
# Dynamical Jahn-Teller effects on the generation of electronic ring currents by circularly polarized light

Krishna R. Nandipati[1,*] and Oriol Vendrell[1,2,†]

[1] *Theoretische Chemie, Physikalisch-Chemisches Institut, Universität Heidelberg, Im Neuenheimer Feld 229, 69120 Heidelberg, Germany*

[2] *Centre for Advanced Materials, Universität Heidelberg, Im Neuenheimer Feld 205, 69120 Heidelberg, Germany*

(Dated: May 21, 2021)

## I. ELECTRONIC RING CURRENTS UNDER VIBRONIC COUPLING OF $(E)$ ELECTRONIC STATES

We consider a molecular system with a symmetry axis $C_n$ of order $n \geq 3$ at the fully symmetric nuclear configuration $\boldsymbol{Q}_0$. This results in the existence of doubly degenerate, diabatic electronic states belonging to an $(E)$ representation of the corresponding symmetry point group. Without loss of generality, we consider as well that the degenerate electronic states are not vibronically coupled to electronic states of other representations, which is the case in the well known $(E \times e)$ Jahn-Teller (JT) Hamiltonian. It is convenient to introduce the complex linear combination of the real-valued $(E)$ electronic states

$$|\Phi_{\pm}(\boldsymbol{Q}_0)\rangle = \frac{1}{\sqrt{2}} \left(|\Phi_x(\boldsymbol{Q}_0)\rangle \pm i|\Phi_y(\boldsymbol{Q}_0)\rangle\right). \tag{1}$$

Using these definitions, the vibronic eigenstates within the subspace of the $(E)$ electronic states can be written as

$$|\Psi_j\rangle = |\Xi_+^{(j)}\rangle \otimes |\Phi_+(\boldsymbol{Q}_0)\rangle + |\Xi_-^{(j)}\rangle \otimes |\Phi_-(\boldsymbol{Q}_0)\rangle, \tag{2}$$

where $|\Xi_\pm^{(j)}\rangle$ is the vibrational contribution of the $j$-th vibronic state associated with the $\pm$-th diabatic electronic state. Our subject of interest is the electronic current $\vec{J}_j(\vec{q})$ related to the electronic charge density via the continuity equation

$$\overset{\bullet}{\rho}_j(\vec{q}) + \vec{\nabla}_q \cdot \vec{J}_j(\vec{q}) = 0, \tag{3}$$

where $\rho_j(\vec{q}) = \langle\Psi_j|\hat{\rho}(\vec{q})|\Psi_j\rangle$. Writing the charge density operator $\hat{\rho}(\vec{q}) = \hat{\psi}^\dagger(\vec{q})\hat{\psi}(\vec{q})$ in terms of field operators, taking its time-derivative and introducing the equation of motion of the field creation and anihilation operators,

$$\begin{aligned}\overset{\bullet}{\hat{\rho}}(\vec{q}) &= \overset{\bullet}{\hat{\psi}}{}^\dagger(\vec{q})\hat{\psi}(\vec{q}) + \hat{\psi}^\dagger(\vec{q})\overset{\bullet}{\hat{\psi}}(\vec{q}) \\ &= \frac{-\hbar}{i2m_e}\left(\hat{\psi}^\dagger(\vec{q})\nabla_q^2\hat{\psi}(\vec{q}) - \left(\nabla_q^2\hat{\psi}^\dagger(\vec{q})\right)\hat{\psi}(\vec{q})\right) \\ &= \frac{-\hbar}{i2m_e}\vec{\nabla}_q\left(\hat{\psi}^\dagger(\vec{q})\vec{\nabla}_q\hat{\psi}(\vec{q}) - \left(\vec{\nabla}_q\hat{\psi}^\dagger(\vec{q})\right)\hat{\psi}(\vec{q})\right),\end{aligned} \tag{4}$$

the current operator

$$\hat{\vec{J}}(\vec{q}) = \frac{\hbar}{i2m_e}\left(\hat{\psi}^\dagger(\vec{q})\vec{\nabla}_q\hat{\psi}(\vec{q}) - \left(\vec{\nabla}_q\hat{\psi}^\dagger(\vec{q})\right)\hat{\psi}(\vec{q})\right) \tag{5}$$

* e-mail: krishna.nandipati@pci.uni-heidelberg.de
† e-mail: oriol.vendrell@uni-heidelberg.de

can be defined. It is now useful to introduce the expansion of the annihilation (creation) field operators in terms of electronic orbital functions, $\hat{\psi}^{(\dagger)} = \sum_l \varphi_l^{(*)} \hat{a}_l^{(\dagger)}$, to arrive at

$$\begin{aligned}\hat{\vec{J}}(\vec{q}) &= \frac{\hbar}{i2m_e} \sum_{lm} \left( \varphi_l^*(\vec{q}) \left( \vec{\nabla}_q \varphi_m(\vec{q}) \right) - \left( \vec{\nabla}_q \varphi_l^*(\vec{q}) \right) \varphi_m(\vec{q}) \right) \hat{a}_l^\dagger \hat{a}_m \\ &= \frac{\hbar}{i2m_e} \sum_{lm} 2i\Im\left\{ \varphi_l^*(\vec{q}) \left( \vec{\nabla}_q \varphi_m(\vec{q}) \right) \right\} \hat{a}_l^\dagger \hat{a}_m \\ &= \frac{1}{m_e} \sum_{lm} \Re\left\{ \varphi_l^*(\vec{q}) \left( \frac{\hbar}{i} \vec{\nabla}_q \varphi_m(\vec{q}) \right) \right\} \hat{a}_l^\dagger \hat{a}_m,\end{aligned} \tag{6}$$

which is the working equation for the current operator. Note that, in the same way as the many-body electronic states, the molecular orbitals are defined at the reference nuclear geometry $\boldsymbol{Q}_0$.

The current can now be obtained as the expectation value of the current operator applied to the full many-body vibronic state

$$\begin{aligned}\langle \Psi_j | \hat{\vec{J}}(\vec{q}) | \Psi_j \rangle &= \langle \Xi_+^{(j)} | \Xi_+^{(j)} \rangle \langle \Phi_+(\boldsymbol{Q}_0) | \hat{\vec{J}}(\vec{q}) | \Phi_+(\boldsymbol{Q}_0) \rangle \\ &+ \langle \Xi_-^{(j)} | \Xi_-^{(j)} \rangle \langle \Phi_-(\boldsymbol{Q}_0) | \hat{\vec{J}}(\vec{q}) | \Phi_-(\boldsymbol{Q}_0) \rangle \\ &+ \langle \Xi_+^{(j)} | \Xi_-^{(j)} \rangle \langle \Phi_+(\boldsymbol{Q}_0) | \hat{\vec{J}}(\vec{q}) | \Phi_-(\boldsymbol{Q}_0) \rangle \\ &+ \langle \Xi_-^{(j)} | \Xi_+^{(j)} \rangle \langle \Phi_-(\boldsymbol{Q}_0) | \hat{\vec{J}}(\vec{q}) | \Phi_+(\boldsymbol{Q}_0) \rangle .\end{aligned} \tag{7}$$

For simplicity, we assume that the $(E)$ configurations of interest are of the form $|\Phi_\pm(\boldsymbol{Q}_0)\rangle = \hat{a}_\pm^\dagger \hat{a}_A |\Phi_0(\boldsymbol{Q}_0)\rangle$, where $|\Phi_0(\boldsymbol{Q}_0)\rangle$ is the fully symmetric, closed shell electronic ground state of the molecule and $\hat{a}_\pm^\dagger \hat{a}_A$ excites an electron from a fully symmetric molecular orbital to an orbital of $(E)$ symmetry. Including further orbitals of $(E)$ symmetry in the excitation leads to the same final expression for the ring current without further insights. The electronic current of the $j$-th vibronic state hence reads

$$\begin{aligned}\vec{J}_j(\vec{q}) = \frac{1}{m_e} \Bigg( &\langle \Xi_+^{(j)} | \Xi_+^{(j)} \rangle \Re\left\{ \varphi_+^*(\vec{q}) \frac{\hbar}{i} \vec{\nabla}_q \varphi_+(\vec{q}) \right\} \\ &+ \langle \Xi_-^{(j)} | \Xi_-^{(j)} \rangle \Re\left\{ \varphi_-^*(\vec{q}) \frac{\hbar}{i} \vec{\nabla}_q \varphi_-(\vec{q}) \right\} \\ &+ \langle \Xi_+^{(j)} | \Xi_-^{(j)} \rangle \Re\left\{ \varphi_+^*(\vec{q}) \frac{\hbar}{i} \vec{\nabla}_q \varphi_-(\vec{q}) \right\} \\ &+ \langle \Xi_-^{(j)} | \Xi_+^{(j)} \rangle \Re\left\{ \varphi_-^*(\vec{q}) \frac{\hbar}{i} \vec{\nabla}_q \varphi_+(\vec{q}) \right\} \Bigg).\end{aligned} \tag{8}$$

Using the symmetry of the $(E)$ MOs, these can be written as

$$\varphi_\pm(\vec{q}; \boldsymbol{Q_0}) = \tilde{\varphi}_E(r, z; \boldsymbol{Q_0}) e^{\pm i\theta} \tag{9}$$

where we use cylindrical coordinates $\vec{q} :\rightarrow (r, z, \theta)$ to describe the electron and where $\tilde{\varphi}_E(r, z; \boldsymbol{Q_0})$ is their real-valued, $\theta$-independent part. Next, we apply the gradient operator in cylindrical coordinates,

$$\vec{\nabla}_q = \frac{\partial}{\partial r} \vec{u}_r + \frac{1}{r} \frac{\partial}{\partial \theta} \vec{u}_\theta + \frac{\partial}{\partial z} \vec{u}_z, \tag{10}$$

to the $(E)$ molecular orbitals

$$\vec{\nabla}_q \varphi_\pm = e^{\pm i\theta} \left( \frac{\partial}{\partial r} \tilde{\varphi}_E \vec{u}_r + \frac{\partial}{\partial z} \tilde{\varphi}_E \vec{u}_z \pm \frac{i}{r} \tilde{\varphi}_E \vec{u}_\theta \right) \tag{11}$$

to obtain the molecular-orbital dependent part of Eq. (8),

$$\varphi_\pm^* \frac{\hbar}{i} \vec{\nabla}_q \varphi_\pm = \frac{\hbar}{i} \left( \tilde{\varphi}_E \frac{\partial}{\partial r} \tilde{\varphi}_E \vec{u}_r + \tilde{\varphi}_E \frac{\partial}{\partial z} \tilde{\varphi}_E \vec{u}_z \right) \pm \frac{\hbar}{r} |\tilde{\varphi}_E|^2 \vec{u}_\theta \tag{12}$$

and,

$$\varphi^*_\mp \frac{\hbar}{i}\vec{\nabla}_q \varphi_\pm = e^{\pm 2i\theta}\left[\frac{\hbar}{i}\left(\tilde{\varphi}_E \frac{\partial}{\partial r}\tilde{\varphi}_E \vec{u}_r + \tilde{\varphi}_E \frac{\partial}{\partial z}\tilde{\varphi}_E \vec{u}_z\right) \pm \frac{\hbar}{r}|\tilde{\varphi}_E|^2 \vec{u}_\theta\right]. \tag{13}$$

Plugging Eqs. (12, 13) into Eq. (8) one arrives at

$$\vec{J}^{(\theta)}_j(\vec{q}) = \frac{\hbar}{m_e r}|\tilde{\varphi}_E|^2\left(\langle \Xi^{(j)}_+|\Xi^{(j)}_+\rangle - \langle \Xi^{(j)}_-|\Xi^{(j)}_-\rangle\right) \tag{14}$$

for the component of the current along the $\theta$-direction. Integrating the $\theta$-component of the current $\vec{J}^{(\theta)}_j(\vec{q})$ along the $r$ and $z$ coordinates and averaging over the $\theta$ coordinate one arrives at the final expression for the *ring* current of the $j$-th vibronic state

$$\begin{aligned}\mathcal{C}_j &= \int_0^\infty r dr \int_{-\infty}^{+\infty} dz \frac{1}{2\pi}\int_0^{2\pi} d\theta \vec{J}^{(\theta)}_j(\vec{q}) \\ &= \frac{\hbar}{m_e}\left(P^{(j)}_+ - P^{(j)}_-\right),\end{aligned} \tag{15}$$

where $P^{(j)}_\pm = \langle \Xi_\pm|\Xi_\pm\rangle$ is the population of the $|\Phi_\pm(\boldsymbol{Q}_0)\rangle$ diabatic electronic state in the $j$-th vibronic state and we used that $\tilde{\varphi}_E$ is normed.

Finally, if one considers the time-dependent Born-Huang expansion [1]

$$|\Psi(t)\rangle = |\Xi_+(t)\rangle \otimes |\Phi_+(\boldsymbol{Q}_0)\rangle + |\Xi_-(t)\rangle \otimes |\Phi_-(\boldsymbol{Q}_0)\rangle \tag{16}$$

instead of the eigenstates (2), the same train of arguments follows straightforwardly and the time-dependent *ring* current of the wavepacket reads

$$\mathcal{C}(t) = \frac{\hbar}{m_e}\left(P_+(t) - P_-(t)\right). \tag{17}$$

## II. COUPLING MATRIX ELEMENTS OF THE $(E \times e)$ JT HAMILTONIAN

The diabatic representation of the $(E \times e)$ JT Hamiltonian up to second-order coupling between the $E$ components reads [2] (in polar coordinates)

$$\begin{aligned}\hat{H} =& \hat{T}_N + \hat{H}_{el} \\ =& \hat{T}_N + \frac{\omega}{2}\rho^2 \boldsymbol{I}_{3\times 3} + \begin{pmatrix} \epsilon_+ & 0 & \kappa\rho e^{-i\alpha} + \frac{1}{2}g\rho^2 e^{2i\alpha} \\ 0 & \epsilon_A & 0 \\ \kappa\rho e^{i\alpha} + \frac{1}{2}g\rho^2 e^{-2i\alpha} & 0 & \epsilon_- \end{pmatrix}\end{aligned} \tag{18}$$

The first order JT coupling matrix elements in the basis $\{|n, m.l\rangle\}$, restricting $l$ to $\pm 1$ for the $E$ states, are as follows [3–5]:

$$\langle n+1, m-1, 1|\kappa\rho e^{-i\alpha}|n, m, -1\rangle = \kappa\sqrt{\frac{n-m+2}{2}} \tag{19a}$$

$$\langle n-1, m-1, 1|\kappa\rho e^{-i\alpha}|n, m, -1\rangle = \kappa\sqrt{\frac{n+m}{2}} \tag{19b}$$

$$\langle n+1, m+1, -1|\kappa\rho e^{i\alpha}|n, m, 1\rangle = \kappa\sqrt{\frac{n+m+2}{2}} \tag{20a}$$

$$\langle n-1, m+1, -1|\kappa\rho e^{i\alpha}|n, m, 1\rangle = \kappa\sqrt{\frac{n-m}{2}} \tag{20b}$$

The second order JT coupling matrix elements in the basis $\{|n,m.l\rangle\}$ are as follows [2, 6]:

$$\langle n+2,m+2,1|\frac{1}{2}g\rho^2e^{2i\alpha}|n,m,-1\rangle = \frac{1}{2}g\sqrt{\frac{n+m+2}{2}}\sqrt{\frac{n+m+4}{2}} \tag{21a}$$

$$\langle n-2,m+2,1|\frac{1}{2}g\rho^2e^{2i\alpha}|n,m,-1\rangle = \frac{1}{2}g\sqrt{\frac{n-m}{2}}\sqrt{\frac{n-m-2}{2}} \tag{21b}$$

$$\langle n,m+2,1|\frac{1}{2}g\rho^2e^{2i\alpha}|n,m,-1\rangle = g\sqrt{\frac{n-m}{2}}\sqrt{\frac{n+m+2}{2}} \tag{21c}$$

$$\langle n+2,m-2,-1|\frac{1}{2}g\rho^2e^{-2i\alpha}|n,m,1\rangle = \frac{1}{2}g\sqrt{\frac{n-m+2}{2}}\sqrt{\frac{n-m+4}{2}} \tag{22a}$$

$$\langle n-2,m-2,-1|\frac{1}{2}g\rho^2e^{-2i\alpha}|n,m,1\rangle = \frac{1}{2}g\sqrt{\frac{n+m}{2}}\sqrt{\frac{n+m-2}{2}} \tag{22b}$$

$$\langle n,m-2,-1|\frac{1}{2}g\rho^2e^{-2i\alpha}|n,m,1\rangle = g\sqrt{\frac{n+m}{2}}\sqrt{\frac{n-m+2}{2}} \tag{22c}$$

## III. EIGENSTATES CURRENT IN THE ($E \times e$) JT MODEL

### A. Linear coupling: $\kappa/\omega \neq 0$ and $g/\omega = 0$

Using 2D-HO basis and employing the above JT coupling matrix elements, the diagonalization of the total Hamiltonian (cf. Eq. 18) gives the eigenstates. These eigenstates are classified by the conserved vibronic angular momentum quantum number $q = 2m + l$ [5], where $m$ and $l$ are the angular momentum quantum numbers of the nuclear $e$ vibration and electronic $E$ state, respectively. For a given $\kappa$, each of the vibronic eigenstate in $q$ block is one-one to degenerate with those of $-q$ block, by the direction-reversal symmetry of $l$ and $m$ [5, 6]. The eigenstates belonging to these blocks are denoted with $|j_{\pm q}\rangle$. We restrict the treatment to $q = 0, \pm 1$ sub-spaces, which limits $l$ quantum number to the lowest-lying $E$ electronic states in molecules (i.e. $\pm 1$) and $m$ to $\{-1, 0, 1\}$.

Using nuclear-electronic basis functions $|n,m,l\rangle$ and limiting $l$ quantum number to the lowest-lying $E$ electronic states in molecules (i.e. $\pm 1$) and $m$ to $\{-1, 0, 1\}$ for arbitrary $n$, the BH expansion of the vibronic eigenstates within $q = \pm 1$ blocks, $|j_{\pm q}\rangle$, is given by [5, 6]

$$|j_{\pm q}\rangle = \sum_{n=\{2k,k\in N_0\}} c^{j_{\pm q}}_{n,0,\pm 1}|n,0,\pm 1\rangle \;+ \sum_{n=\{2k+1,k\in N_0\}} c^{j_{\pm q}}_{n,\pm 1,\mp 1}|n,\pm 1,\mp 1\rangle. \tag{23}$$

Fixing $q = +1$, for example, the population of each ring-current direction is, accordingly,

$$P^{(j_{+1})}_{+} = \sum_{n=\{2k,k\in N_0\}} |c^{j_{+1}}_{n,0,1}|^2 \tag{24}$$

$$P^{(j_{+1})}_{-} = \sum_{n=\{2k+1,k\in N_0\}} |c^{j_{+1}}_{n,1,-1}|^2 \tag{25}$$

In general, $P^{(j_{+1})}_{+} \neq P^{(j_{+1})}_{-}$, and according to Eq. (15) there is a net imbalance in the total contributions of the electronic $E_+$ ($l$=1) and $E_-$ ($l$=-1) states in a given vibronic eigenstate. The general features of the currents supported by the eigenstates are discussed in the main text with an application to sym-triazine.

### B. Linear plus quadratic coupling: $\kappa/\omega \neq 0$ and $g/\omega \neq 0$

The presence of second-order JT coupling hinders nuclear pseudorotation on the lower sheet of the "Mexican hat" potentials, due to the development of three minima separated by three saddle points. Under second order coupling, $q$ is not a good quantum number anymore because the total vibronic angular momentum does not commute with the Hamiltonian. Nonetheless, the eigenstates still separate into two degenerate blocks due to the overall rotational symmetry of the system, which can be seen by inspecting the second-order couplings in Eqs. (22a,21a). The degenerate

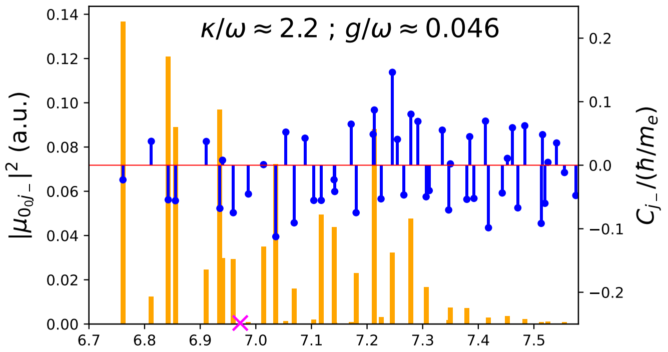


FIG. 1. Absorption spectrum ($\propto |\mu_{0_0 j_-}|^2$) for the 2D sym-triazine ($E \times e$) JT Hamiltonian with inclusion of second-order JT coupling (orange, left y-scale) and eigenstate ring currents ($\mathcal{C}_{j_-}/(\hbar/m_e)$) (blue, right y-scale) as a function of the eigenstates' energy.

eigenstate in one of the two blocks is still obtained by changing the sign of the $m$ and $l$ quantum numbers in all basis states of the corresponding eigenstate of the other block [6]. This corresponds to changing the direction of rotation of all particles.

For completeness, we show in Fig. 1 the calculated absorption spectrum for sym-triazine system with inclusion of second-order JT coupling ( $g/\omega = 0.046$) [6]. The spectrum retains its gross features due to dominant first-order JT coupling ($\kappa/\omega = 2.2$, cf. Fig. 2a-b in the main text) but develops splittings in some of the main intense lines. Obviously, the spectrum has more lines than its linear JT counterpart as the basis states belonging to different q-blocks now participate in the coupling mechanism. The net currents associated with the optically bright states are also shown in the figure. There occur eigenstates at various spectral regions supporting either circulation direction of the electrons, similar to the Fig. 2a-b in the main text (i.e. when $\kappa/\omega = 2.2$ and $g/\omega = 0$). The circulation direction of the electrons still depends on the eigenstates and the corresponding spectral region. Therefore, even in the presence couplings beyond first order it is still possible to determine the direction of the ring-current depending on the wavelength of the circularly polarized photons.


[1] M. Born and K. Huang, *Dynamical theory of crystal lattices* (Clarendon press, 1954).
[2] I. B. Bersuker, *The Jahn-Teller effect* (Cambridge University Press, 2006).
[3] W. Moffitt and A. Liehr, Configurational instability of degenerate electronic states, Phys. Rev. **106**, 1195 (1957).
[4] G. Gallup, Matrix elements and eigenfunctions of multidimensional oscillators by operational methods: Part i. two dimensional isotropic harmonic oscillator, J. Mol. Spectrosc. **3**, 148 (1959).
[5] H. C. Longuet-Higgins, U. Öpik, M. H. L. Pryce, and R. A. Sack, Studies of the Jahn–Teller effect .II. The dynamical problem, Proc. R. Soc. A **244**, 1 (1958).
[6] R. L. Whetten, K. S. Haber, and E. R. Grant, The dynamic jahn–teller effect in sym-triazine: Nonadiabatic wave functions and hindered fluxionality, J. Chem. Phys. **84**, 1270 (1986).
